# Supplementary material for: Molecular Density Functional Theory for water with liquid-gas coexistence and correct pressure
Source: arXiv:1502.03048 ancillary file (2015-04-18)
Supplement: Supplementary file 1 [file SuppInfo.pdf]

# Supplementary informations for "Molecular Density Functional Theory for water with liquid-gas coexistence and correct pressure"

Guillaume Jeanmairet, Maximilien Levesque, Volodymyr Sergiievskyi and Daniel Borgis

## I. REWRITING OF THE BRIDGE FUNCTIONAL AS A WEIGHTED DENSITY FUNCTIONAL

We start from the expression of the three-body bridge correction in Eq.1. In order to reduce the computational cost of its evaluation, we rewrite it in terms of 7 scalars and 1 vectorial convolution products:

$$\beta\mathcal{F}_{3\mathrm{B}}[n(\boldsymbol{r})] = \frac{\lambda}{2}\int \Delta n(\boldsymbol{r}_1)\Bigg[\iint \Delta n(\boldsymbol{r}_2)\Delta n(\boldsymbol{r}_3) f(r_{12}) f(r_{13}) \times \left(\frac{\boldsymbol{r}_{12}\cdot\boldsymbol{r}_{13}}{r_{12}r_{13}} - \cos\theta_0\right)^2 \mathrm{d}\boldsymbol{r}_2\mathrm{d}\boldsymbol{r}_3\Bigg]\mathrm{d}\boldsymbol{r}_1, \tag{1}$$

where the double integration in the squared parenthesis in Eq.1 is a function of $\boldsymbol{r}_1$. We define $G$:

$$G(\boldsymbol{r}_1) = \iint \Delta n(\boldsymbol{r}_2)\Delta n(\boldsymbol{r}_3) f(r_{12}) f(r_{13}) \left(\frac{\boldsymbol{r}_{12}\cdot\boldsymbol{r}_{13}}{r_{12}r_{13}} - \cos\theta_0\right)^2 \mathrm{d}\boldsymbol{r}_2\mathrm{d}\boldsymbol{r}_3, \tag{2}$$

and we expand it:

$$G(\boldsymbol{r}_1) = \iint \Delta n(\boldsymbol{r}_2)\Delta n(\boldsymbol{r}_3) f(r_{12}) f(r_{13}) \left[\left(\frac{\boldsymbol{r}_{12}\cdot\boldsymbol{r}_{13}}{r_{12}r_{13}}\right)^2 - 2\cos\theta_0\frac{\boldsymbol{r}_{12}\cdot\boldsymbol{r}_{13}}{r_{12}r_{13}} + \cos^2\theta_0\right] \mathrm{d}\boldsymbol{r}_2\mathrm{d}\boldsymbol{r}_3. \tag{3}$$

Then, one splits $G$ in a sum of three functions, $H_0$, $H_1$ and $H_2$:

$$G(\boldsymbol{r}_1) = H_2(\boldsymbol{r}_1) + H_1(\boldsymbol{r}_1) + H_0(\boldsymbol{r}_1), \tag{4}$$

where

$$H_2(\boldsymbol{r}_1) = \iint \Delta n(\boldsymbol{r}_2)\Delta n(\boldsymbol{r}_3) f(r_{12}) f(r_{13}) \left(\frac{\boldsymbol{r}_{12}\cdot\boldsymbol{r}_{13}}{r_{12}r_{13}}\right)^2 \mathrm{d}\boldsymbol{r}_2\mathrm{d}\boldsymbol{r}_3, \tag{5}$$

$$H_1(\boldsymbol{r}_1) = -2\cos\theta_0 \iint \Delta n(\boldsymbol{r}_2)\Delta n(\boldsymbol{r}_3) f(r_{12}) f(r_{13}) \frac{\boldsymbol{r}_{12}\cdot\boldsymbol{r}_{13}}{r_{12}r_{13}} \mathrm{d}\boldsymbol{r}_2\mathrm{d}\boldsymbol{r}_3, \tag{6}$$

and

$$H_0(\boldsymbol{r}_1) = \cos^2(\theta_0) \iint \Delta n(\boldsymbol{r}_2)\Delta n(\boldsymbol{r}_3) f(r_{12}) f(r_{13}) \mathrm{d}\boldsymbol{r}_2\mathrm{d}\boldsymbol{r}_3. \tag{7}$$

For the sake of clarity, the indices of $H_i$ denotes the tensorial order of the integrand.

Since $\boldsymbol{r}_2$ and $\boldsymbol{r}_3$ are independent in Eq.7, the separation of the two integrals is straightforward:

$$H_0(\boldsymbol{r}_1) = \cos^2(\theta_0)\left[\int \Delta n(\boldsymbol{r}_2) f(r_{12}) \mathrm{d}\boldsymbol{r}_2\right]^2 = \cos^2(\theta_0)\, \bar{n}_0(r_1)^2, \tag{8}$$

with

$$\bar{n}_0(\boldsymbol{r}_1) = \int f(r_{12}) \Delta n(\boldsymbol{r}_2) \mathrm{d}\boldsymbol{r}_2. \tag{9}$$

We now focus on $H_1$. This function can be rewritten by using the cartesian coordinates $(x, y, z)$ for the dot product:

$$H_1(\boldsymbol{r}_1) = -2\cos\theta_0 \iint \Delta n(\boldsymbol{r}_2)\Delta n(\boldsymbol{r}_3) f(r_{12}) f(r_{13}) \sum_{\alpha\in\{x,y,z\}} \frac{\alpha_{12}\alpha_{13}}{r_{12}r_{13}} \mathrm{d}\boldsymbol{r}_2 \mathrm{d}\boldsymbol{r}_3. \tag{10}$$

Since the 2 and 3 variables are independent,

$$H_1(\boldsymbol{r}_1) = -2\cos\theta_0 \sum_{\alpha\in\{x,y,z\}} \int \Delta n(\boldsymbol{r}_2) f(r_{12}) \frac{\alpha_{12}}{r_{12}} \left[\int \Delta n(\boldsymbol{r}_3) f(r_{13}) \frac{\alpha_{13}}{r_{13}} \mathrm{d}\boldsymbol{r}_3\right] \mathrm{d}\boldsymbol{r}_2 \tag{11}$$

The expressions in square bracket are functions of $\boldsymbol{r}_1$, not of $\boldsymbol{r}_2$, that is taken out of the outer integral. This gives

$$H_1(\boldsymbol{r}_1) = -2\cos\theta_0 \sum_{\alpha\in\{x,y,z\}} \bar{\boldsymbol{n}}_1(\boldsymbol{r}_1) \cdot \boldsymbol{u}_\alpha \int \Delta n(\boldsymbol{r}_2) f(r_{12}) \frac{\alpha_{12}}{r_{12}} \mathrm{d}\boldsymbol{r}_2, \tag{12}$$

where $\boldsymbol{u}_\alpha$ is the unitary vector pointing along direction $\alpha$ and

$$\bar{\boldsymbol{n}}_1(\boldsymbol{r}_1) = \int f(r_{13}) \frac{\boldsymbol{r}_{13}}{r_{13}} \Delta n(\boldsymbol{r}_3) \mathrm{d}\boldsymbol{r}_3. \tag{13}$$

The remaining integrals in Eq.12 are the same functions of $\boldsymbol{r}_1$ than the one in pre-factor. Finally,

$$H_1(\boldsymbol{r}_1) = -2\cos\theta_0 \sum_{\alpha\in\{x,y,z\}} (\Delta\boldsymbol{n}_1(\boldsymbol{r}_1) \cdot \boldsymbol{u}_\alpha)^2 = -2\cos\theta_0 \bar{\boldsymbol{n}}_1(\boldsymbol{r}_1) \cdot \bar{\boldsymbol{n}}_1(\boldsymbol{r}_1) \tag{14}$$

We use a similar strategy for $H_2$. First we expand the function by using the cartesian coordinates in the dot product:

$$H_2(\boldsymbol{r}_1) = \iint \Delta n(\boldsymbol{r}_2)\Delta n(\boldsymbol{r}_3) f(r_{12}) f(r_{13}) \left[\sum_{\alpha\in\{x,y,z\}} \frac{\alpha_{12}\alpha_{13}}{r_{12}r_{13}}\right]^2 \mathrm{d}\boldsymbol{r}_2 \mathrm{d}\boldsymbol{r}_3. \tag{15}$$

The square parenthesis can be rewritten:

$$\left[\sum_{\alpha\in\{x,y,z\}} \frac{\alpha_{12}\alpha_{13}}{r_{12}r_{13}}\right]^2 = \sum_{\alpha\in\{x,y,z\}} \sum_{\beta\in\{x,y,z\}} \frac{\alpha_{12}\alpha_{13}\beta_{12}\beta_{13}}{r_{12}^2 r_{13}^2}. \tag{16}$$

We apply the same separation of $\boldsymbol{r}_2$ and $\boldsymbol{r}_3$:

$$H_2(\boldsymbol{r}_1) = \sum_{\alpha\in\{x,y,z\}} \sum_{\beta\in\{x,y,z\}} \int \Delta n(\boldsymbol{r}_2) f(r_{12}) \frac{\alpha_{12}\beta_{12}}{r_{12}^2} \left[ \int \Delta n(\boldsymbol{r}_3) f(r_{13}) \frac{\alpha_{13}\beta_{13}}{r_{13}^2} \mathrm{d}\boldsymbol{r}_3 \right] \mathrm{d}\boldsymbol{r}_2. \quad (17)$$

By introducing the functions of $\boldsymbol{r}_1$, $\Delta n_{\alpha\beta}$, already defined in the article as,

$$\bar{n}_{\alpha\beta}(\boldsymbol{r}_1) = \int f(r_{12}) \frac{\alpha_{12}\beta_{12}}{r_{12}^2} \Delta n(\boldsymbol{r}_2) \mathrm{d}\boldsymbol{r}_2, \text{ with } \alpha \text{ and } \beta = x \text{ or } y \text{ or } z, \quad (18)$$

we get a final expression for $H_2$:

$$H_2(\boldsymbol{r}_1) = \sum_{\alpha,\beta\in\{x,y,z\}} \bar{n}_{\alpha\beta}(\boldsymbol{r}_1)^2. \quad (19)$$

Inserting Eq.19, Eq.14, and Eq. 8 in Eq.4, we find that Eq.1 and Eq.20 are equivalent:

$$\beta\mathcal{F}_{3\mathrm{B}}[n(\boldsymbol{r})] = \frac{\lambda}{2} \int \Delta n(\boldsymbol{r}_1) \left[ \sum_{\alpha,\beta\in\{x,y,z\}} \bar{n}_{\alpha\beta}(\boldsymbol{r}_1)^2 + \cos^2(\theta_0)\, \bar{n}_0(\boldsymbol{r}_1)^2 - 2\cos(\theta_0)\, \bar{\boldsymbol{n}}_1(\boldsymbol{r}_1) \cdot \bar{\boldsymbol{n}}_1(\boldsymbol{r}_1) \right] \mathrm{d}\boldsymbol{r}_1. \quad (20)$$

## II. FIRST- AND SECOND-ORDER FUNCTIONAL DERIVATIVES OF THE THREE-BODY BRIDGE FUNCTIONAL

One usually needs first and second-order functional derivatives to minimize the functional. The first-order functional derivative of the bridge functional reads

$$\left.\frac{\beta\delta\mathcal{F}_{3\mathrm{B}}[n(\boldsymbol{r})]}{\delta n(\boldsymbol{r})}\right|_{\boldsymbol{r}=\boldsymbol{r}_1} = \frac{1}{2}\lambda \iint f(r_{12}) f(r_{13}) \left( \frac{\boldsymbol{r}_{12}\cdot\boldsymbol{r}_{13}}{r_{12}r_{13}} - \cos\theta_0 \right)^2 \Delta n(\boldsymbol{r}_2)\Delta n(\boldsymbol{r}_3) \mathrm{d}\boldsymbol{r}_2 \mathrm{d}\boldsymbol{r}_3 + \lambda \int \Delta n(\boldsymbol{r}_2) \left[ \int f_w(r_{12}) f_w(r_{23}) \left( \frac{\boldsymbol{r}_{12}\cdot\boldsymbol{r}_{23}}{r_{12}r_{23}} - \cos\theta_0 \right)^2 \Delta n(\boldsymbol{r}_3) \mathrm{d}\boldsymbol{r}_3 \right] \mathrm{d}\boldsymbol{r}_2. \quad (21)$$

It can be re-expressed, by virtue of the three previous demonstrations:

$$\left.\frac{\beta\delta\mathcal{F}_{3\mathrm{B}}[n(\boldsymbol{r})]}{\delta n(\boldsymbol{r})}\right|_{\boldsymbol{r}=\boldsymbol{r}_1} = \frac{1}{2}\lambda \left[ \sum_{\alpha,\beta\in\{x,y,z\}} \bar{n}_{\alpha\beta}(\boldsymbol{r}_1)^2 + \cos^2(\theta_0)\, \bar{n}_0(\boldsymbol{r}_1)^2 - 2\cos(\theta_0)\, \bar{\boldsymbol{n}}_1(\boldsymbol{r}_1)\cdot\bar{\boldsymbol{n}}_1(\boldsymbol{r}_1) \right] + \lambda \int \Delta n(\boldsymbol{r}_2) f(r_{12}) \left[ \sum_{\alpha,\beta\in\{x,y,z\}} \bar{n}_{\alpha\beta}(\boldsymbol{r}_1) \frac{\alpha_{12}\beta_{12}}{r_{12}^2} + \cos^2(\theta_0)\, \bar{n}_0(\boldsymbol{r}_1) - 2\cos(\theta_0)\, \bar{\boldsymbol{n}}_1(\boldsymbol{r}_1)\cdot \frac{\boldsymbol{r}_{12}}{r_{12}} \right] \mathrm{d}\boldsymbol{r}_2. \quad (22)$$

The second-order functional derivative of Eq.1 reads

$$\left.\frac{\beta\delta^2\mathcal{F}_{3\mathrm{B}}[n(\boldsymbol{r})]}{\delta n(\boldsymbol{r})\delta n(\boldsymbol{r}')}\right|_{\boldsymbol{r}=\boldsymbol{r}_1;\boldsymbol{r}'=\boldsymbol{r}_2} = \lambda\int f(r_{12})f(r_{13})\left(\frac{\boldsymbol{r}_{12}\cdot\boldsymbol{r}_{13}}{r_{12}r_{13}}-\cos\theta_0\right)^2\Delta n(\boldsymbol{r}_3)\mathrm{d}\boldsymbol{r}_3$$
$$+\lambda\int f(r_{12})f(r_{23})\left(\frac{\boldsymbol{r}_{12}\cdot\boldsymbol{r}_{23}}{r_{12}r_{23}}-\cos\theta_0\right)^2\Delta n(\boldsymbol{r}_3)\mathrm{d}\boldsymbol{r}_3$$
$$+\lambda\int f(r_{13})f(r_{23})\left(\frac{\boldsymbol{r}_{13}\cdot\boldsymbol{r}_{23}}{r_{13}r_{23}}-\cos\theta_0\right)^2\Delta n(\boldsymbol{r}_3)\mathrm{d}\boldsymbol{r}_3. \tag{23}$$
